# Supplementary material for: Data-Driven Track Following Control for Dual Stage-Actuator Hard Disk Drives
Source: arXiv:2304.00720 source file (2023-04-03)
Supplement: Supplementary file 1 [file Appendix.tex]

\section{$H_\infty$ Constraints}
\begin{figure}[ht!]
\begin{center}
\includegraphics[width=8.4cm]{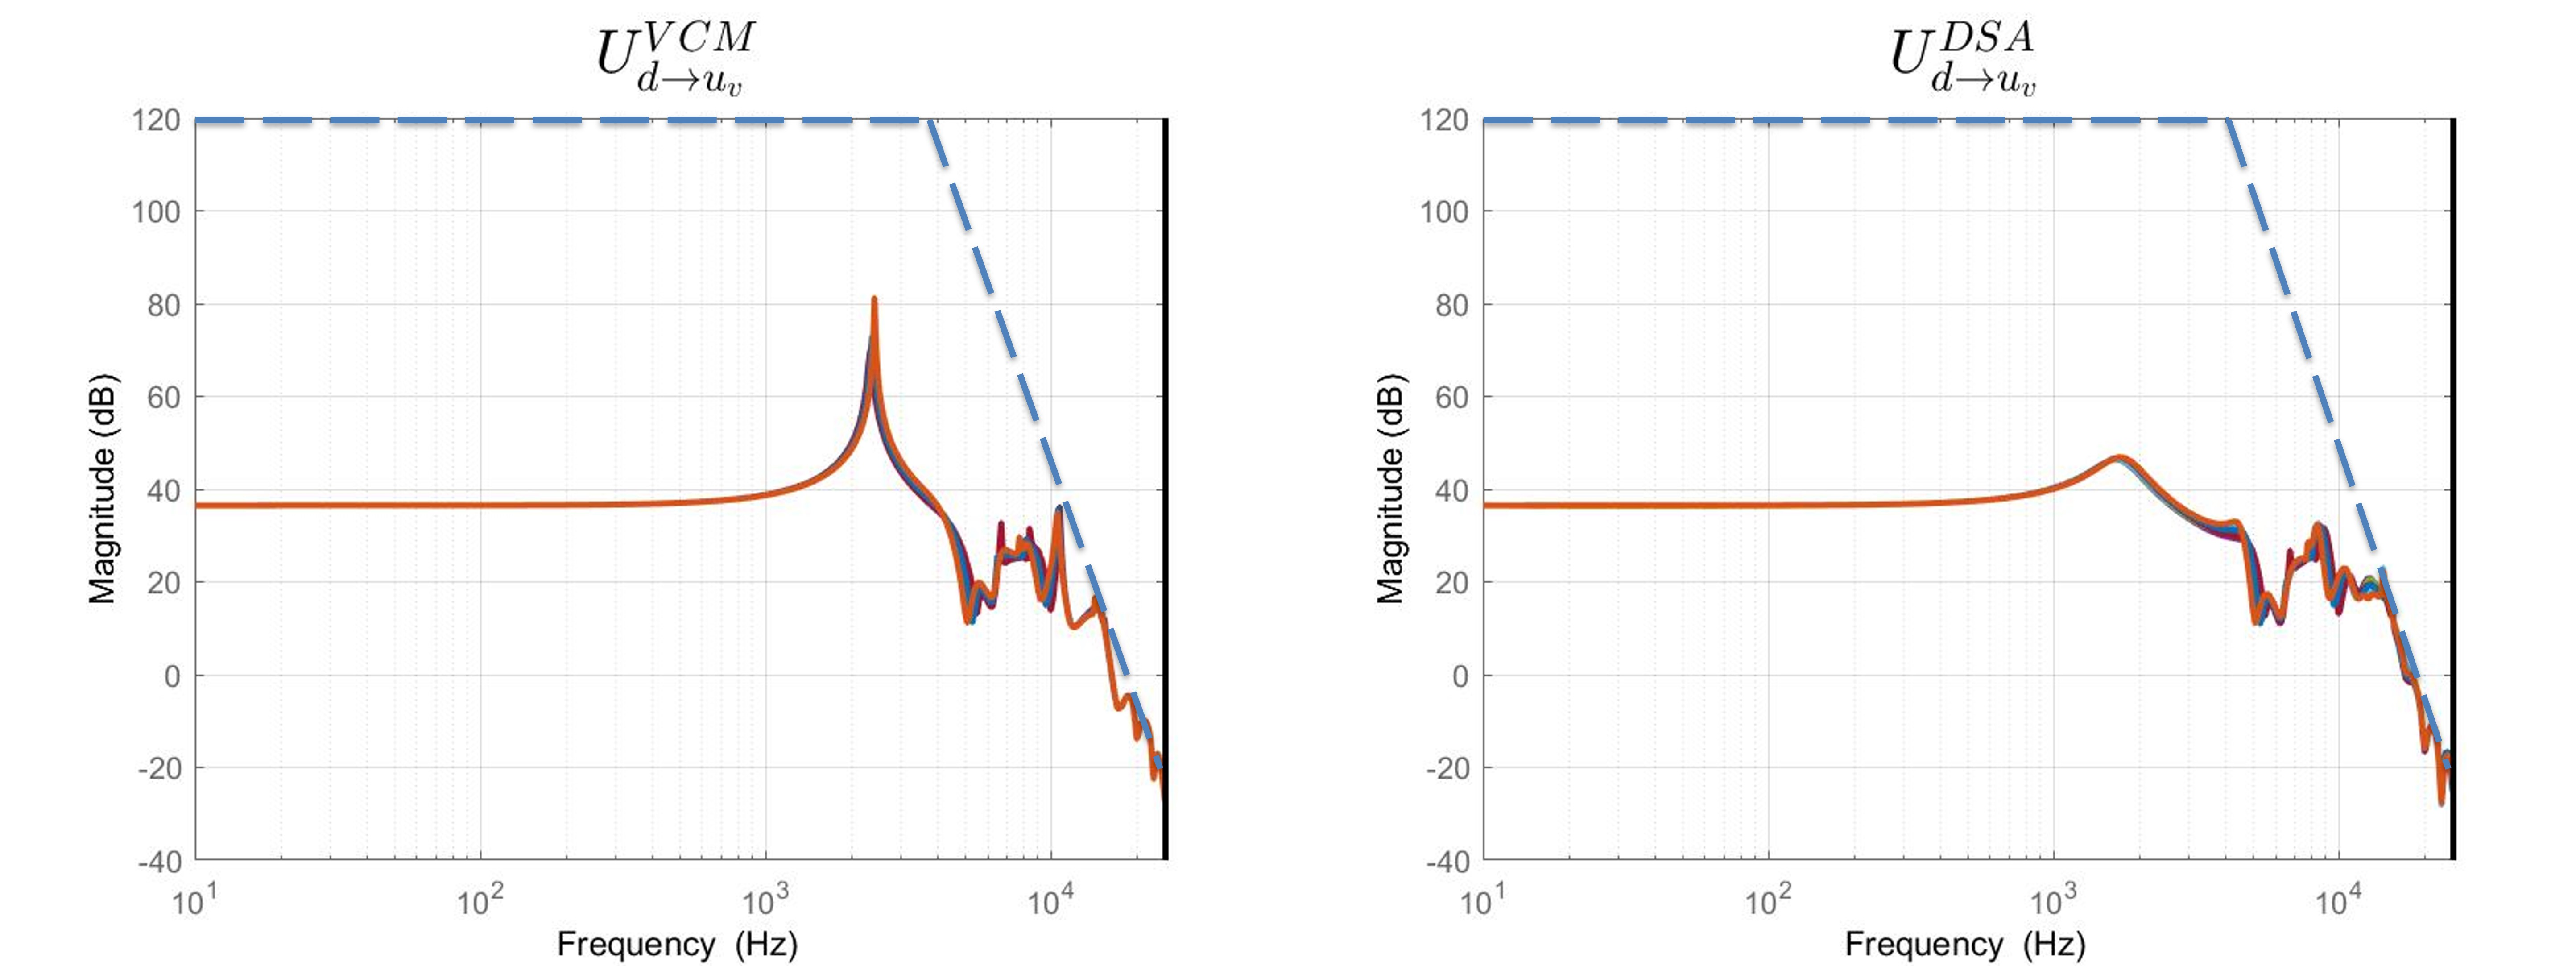}
\caption{This image was uploaded to writeLaTeX via the project menu.}
\label{fig:PZTFR}
\end{center}
\end{figure}
